# Supplementary material for: Research-Oriented Human-Centric Evaluation for Foundation Models
Source: arXiv:2506.01793 source file (2026-08-14)
Supplement: Supplementary file 1 [file appendix.tex]

\section{Appendix}

\subsection{Tasks in the experiments}\label{sec:tasks}

\begin{table*}
  \caption{Examples of Different Task Types Across Disciplines}
  \label{tab:tasks}
  \begin{tabularx}{\textwidth}{p{2.5cm} p{5cm} p{9cm}}
    \toprule
    \textbf{Domain} & \textbf{Literature Synthesis Problems} & \textbf{Innovation-Driven Problems} \\
    \midrule
    Computer Science & 
    Survey on generative image quality evaluation & 
    How to enhance collaboration and game-playing capabilities among AI agents in multi-agent systems to approach human collective intelligence? \\
    
    Legal Studies & 
    Literature review on the justification of legal enforcement of morality & 
    How should legal frameworks balance medical innovation and ethical regulation in the CRISPR-enabled future of genetic engineering? \\
    
    Economics & 
    Market performance analysis of ESG investment strategies in financial sector (past 5 years) & 
    How to improve risk hedging mechanisms in modern derivative markets to mitigate systemic financial crisis risks? \\ 
    
    Healthcare & 
    Feasibility analysis of multimodal diagnostic systems in clinical practice & 
    How to optimize drug delivery systems for enhanced efficacy and reduced adverse effects? \\
    
    Social Sciences & 
    Proposal for a basic metaverse framework & 
    How to balance press freedom and disinformation governance in the digital era? \\
    
    Environmental Science & 
    Long-term biodiversity impact study of climate engineering & 
    How to design sustainable agricultural production models under climate change constraints? \\
    
    Biology & 
    Ecosystem impact assessment of gene drive technology & 
    How to investigate human gut microbiome's role in health/disease and develop targeted interventions? \\
    
    Education & 
    Feasibility study of VR technology in immersive pedagogy & 
    How to construct lifelong learning ecosystems for continuous competency development? \\
    \bottomrule
  \end{tabularx}
\end{table*}

\subsection{Statistic Analysis}

We need to validate the rationality of the experimental design through statistical analysis. In this paper, we use \textbf{Pearson correlation analysis} to verify the validity of the evaluation dimensions and apply the \textbf{Bootstrap algorithm} to assess whether the sample size is sufficient.

To conduct statistical analysis, we selected a small number of tasks and performed a large number of trials to obtain sample data for validating the experimental design. Specifically, we chose Literature Synthesis Problems from three domains: law, sociology, and environment engineering. Evaluators interacted with Deepseek R1, GPT-3 mini, and Grok-3, conducting 10 trials per task in Chinese contexts and 5 trials per task in English contexts for the same model and task. This resulted in a total of 135 sample data points, which were then subjected to the following statistical analyses.

\subsubsection{Validity of the evaluation dimensions}
The Pearson correlation coefficient is calculated based on the covariance and standard deviations of two variables. For two specified dimensions $X$ and $Y$, the Pearson correlation coefficient $r_{xy}$ is defined as:

\begin{equation}
r_{xy}=\frac{\sum_{i=1}^N(x-\bar{x})(y-\bar{y})}{\sqrt{\sum_{i=1}^N(x_i-\bar{x})^2}\sqrt{\sum_{i=1}^N(y_i-\bar{y})^2}}
\end{equation}

where $N$ represents the total number of evaluation records, $x_i$, $y_i$ denote the scores of the i-th evaluation record in dimensions $X$ and $Y$, respectively, $\bar{x}$, $\bar{y}$ are the mean scores across all evaluation records.

The value of the Pearson correlation coefficient $r_{xy}$ ranges between $[-1,1]$. The closer the absolute value is to 1, the stronger the linear correlation; the closer it is to 0, the weaker the linear correlation.
